# Supplementary material for: Joint Spatio-Textual Reasoning for Answering Tourism Questions
Source: arXiv:2009.13613 source file (2020-10-19)
Supplement: Supplementary file 1 [file appendix.tex]

The train data consists of 500 negative samples for each question (75\% hard, 25\% soft). The universe size for the test data is approximately 1250 ranging from 10 to 16200.

\begin{table}[H]
\scriptsize
\centering
\begin{tabular}{|l|l|l|l|l|l|l|}
\hline
\multicolumn{1}{|c|}{\textbf{}} & \multicolumn{2}{c|}{\textbf{Location}} & \multicolumn{2}{c|}{\textbf{Non-location}} \\ \hline
\multicolumn{1}{|c|}{\textbf{Dataset}} & \multicolumn{1}{c|}{\textbf{Questions}} & \multicolumn{1}{c|}{\textbf{QA pairs}} & \multicolumn{1}{c|}{\textbf{Questions}} & \multicolumn{1}{c|}{\textbf{QA pairs}} \\ \hline
Train & 9,617 & 21,396 & 10,342 & 22,150 \\ \hline
Dev & 1,065 & 2,209 & 1,054 & 1,987 \\ \hline
Test & 1,086 & 2,198 & 1,087 & 2,144 \\ \hline
\end{tabular}
\caption{Distribution of questions with location-mention across train, dev \& test sets.}
\label{tab:loc-stats-table}
\end{table}

\begin{table}[H]
\scriptsize
\centering
\begin{tabular}{|l|l|l|l|l|l|l|}
\hline
\multicolumn{1}{|c|}{\textbf{}} & \multicolumn{2}{c|}{\textbf{Correctly Answered}} & \multicolumn{2}{c|}{\textbf{Incorrectly Answered}} \\ \hline
\multicolumn{1}{|c|}{\textbf{Bucket size}} & \multicolumn{1}{c|}{\textbf{Questions}} & \multicolumn{1}{c|}{\textbf{Percentage}} & \multicolumn{1}{c|}{\textbf{Questions}} & \multicolumn{1}{c|}{\textbf{Percentage}} \\ \hline
0-200      & 318 & 26.39\% & 42 & 14.24\%  \\  \hline
200-500    & 417 & 34.61\% & 83 & 28.13\% \\ \hline
500-1000   & 221 & 18.34\% & 53 & 17.97\% \\ \hline
1000-5000  & 178 & 14.77\% & 82 & 27.80\% \\ \hline
5000-20000 & 71  & 5.89\%  & 35 & 11.86\% \\ \hline
\end{tabular}
\caption{Performance of Spatial Net. decreases with increase in universe size.}
\label{tab:toy-error-table1}
\end{table}

% \begin{table}[H]
% \scriptsize
% \centering
% \begin{tabular}{|l|l|l|l|l|l|l|}
% \hline
% \multicolumn{1}{|c|}{\textbf{}} & \multicolumn{2}{c|}{\textbf{Correctly Answered}} & \multicolumn{2}{c|}{\textbf{Incorrectly Answered}} \\ \hline
% \multicolumn{1}{|c|}{\textbf{Bucket size}} & \multicolumn{1}{c|}{\textbf{Questions}} & \multicolumn{1}{c|}{\textbf{Percentage}} & \multicolumn{1}{c|}{\textbf{Questions}} & \multicolumn{1}{c|}{\textbf{Percentage}} \\ \hline
% 0-0.0001    & 85  & 7.05\%  & 153 & 51.86\%  \\  \hline
% 0.0001-0.01 & 234 & 19.42\% & 111 & 37.63\%  \\ \hline
% 0.01-1.0    & 503 & 41.74\% & 25  & 8.48\%   \\ \hline
% 1.0-100.0   & 383 & 31.78\% & 6   & 2.03\%   \\ \hline
% \end{tabular}
% \caption{Performance of Spatial Net. decreases with decrease in the difference of cumulative score of the best and second best candidates.}
% \label{tab:toy-error-table2}
% \end{table}

\begin{table}[H]
\scriptsize
\centering
\begin{tabular}{|l|l|l|l|l|l|l|}
\hline
\multicolumn{1}{|c|}{\textbf{}} & \multicolumn{2}{c|}{\textbf{Correctly Answered}} & \multicolumn{2}{c|}{\textbf{Incorrectly Answered}} \\ \hline
\multicolumn{1}{|c|}{\textbf{Size}} & \multicolumn{1}{c|}{\textbf{Questions}} & \multicolumn{1}{c|}{\textbf{Percentage}} & \multicolumn{1}{c|}{\textbf{Questions}} & \multicolumn{1}{c|}{\textbf{Percentage}} \\ \hline
1 & 233 & 19.34\%  & 0  & 0.00\%  \\  \hline
2 & 671 & 55.69\% & 126 & 42.71\% \\ \hline
3 & 301 & 24.98\% & 169 & 57.29\% \\ \hline
\end{tabular}
\caption{Performance of Spatial Net. decreases with increase in the number of location mentions in the question.}
\label{tab:toy-error-table2}
\end{table}

\begin{table}[H]
\scriptsize
\center
\begin{tabular}{|c|l|l|l|l|l|}
\hline
\multicolumn{1}{|l|}{}                                          & \multicolumn{5}{|c|}{Location Questions}                                \\ \hline
\multicolumn{1}{|c|}{\bf Models}                                          & \textbf{Acc@3} & \textbf{Acc@5} & {\bf Acc@30} & \textbf{MRR} & \textbf{Dg} \\\hline
%SD                                                            &           2.49    &       3.41       &  14.29   &    0.029     &       3.07      \\ \hline
%LocNet                                                        &                &                &      &        &             \\ \hline \hline
$\cs$                                                          &      15.84          &     20.26        &  {\bf 51.47}    &   0.149    &      2.61      \\ \hline
$\cs$ $\rightarrow$ SD        &   11.34             &   17.26     &   {\bf 51.47}     &      0.118        & {\bf 2.18}             \\ \hline
$\cs$ $\rightarrow$ LocNet     &      8.38          &  13.72     &  {\bf 51.47}       & 0.097                &    2.27         \\ \hline 
$\csr$ & 19.89 & 26.43 & {\bf 51.47} & 0.168 & 2.70 \\ \hline
\begin{tabular}[c]{@{}c@{}}Spatio-textual\\ CSRQA\end{tabular} 
& {\bf 21.36} & {\bf 28.36} & {\bf 51.47} & {\bf 0.183} & 2.27 \\ \hline
\multicolumn{1}{|l|}{}                                          & \multicolumn{5}{|c|}{All Questions}                                \\ \hline
%\multicolumn{1}{|c|}{\bf Models}                                          & \textbf{Acc@3} & \textbf{Acc@5} & {\bf Acc@30} & \textbf{MRR} & \textbf{Dg} \\\hline
%SD                                                            &           2.49    &       3.41       &  14.29   &    0.029     &       3.07      \\ \hline
%LocNet                                                        &                &                &      &        &             \\ \hline \hline
%$\cs$                                                          &      15.84          &     20.26        &  51.47    &   0.149    &      2.61      \\ \hline
%$\cs$ $\rightarrow$ SD        &   11.34             &   17.26     &   51.47     &      0.118        & 2.18             \\ \hline
%$\cs$ $\rightarrow$ LocNet     &      8.38          &  13.72     &  51.47       & 0.097                &    2.27         \\ \hline \hline

$\csr$ & 21.45 & 28.21 & {\bf 52.65} & 0.186 & 2.47 \\ \hline
\begin{tabular}[c]{@{}c@{}}Spatio-textual\\ CSRQA\end{tabular} 
& {\bf 22.41} & {\bf 28.99} & {\bf 52.65} & {\bf 0.193} & {\bf 2.32}\\ \hline

\end{tabular}

\caption{Comparison of re-ranking models operating on a reduced search space returned by $\cs$ on Location Questions (ii) Comparison with current state-of-the-art $\csr$ on the full task.} %The $\csr$ model is a $\cs$ $\rightarrow$ $\crq$ model and the 
%Spatio-textual $\csr$ refers to re-ranking using the spatio-textual $\crq$ instead of $\crq$.} % joint Spatio-Textual models with pipe-lined baselines using SD (Sort-by-distance) and Location Reasoning (LocNET) on questions that have location mentions} 
\label{tab:csr-loc-results}
\end{table}

\begin{table}[H]
\begin{tabular}{cc}
\textbf{Error type}                                                                & \textbf{Percentage}      \\
Distractor                                                                         & \textit{12.6}            \\
\begin{tabular}[c]{@{}c@{}}Far-from required\\ location\end{tabular}               & \textit{22.3}            \\
\begin{tabular}[c]{@{}c@{}}Not in requested \\ neighbourhood\\  /area\end{tabular} & \textit{10.7}            \\
\begin{tabular}[c]{@{}c@{}}Location-tagging \\ error\end{tabular}                  & 5.8                      \\
\begin{tabular}[c]{@{}c@{}}Location names\\  repeated\end{tabular}                 & 4.9                      \\
\begin{tabular}[c]{@{}c@{}}Error in \\ Geo-spatial data\end{tabular}               & \multicolumn{1}{l}{2.9}  \\
\begin{tabular}[c]{@{}c@{}}Textual-Reasoning\\  Error\end{tabular}                 & \multicolumn{1}{l}{37.9} \\
\multicolumn{1}{l}{Invalid Question}                                               & \multicolumn{1}{l}{2.9} 
\end{tabular}
\end{table}
\section{Reproducibility Checklist}
Computing Infrastructure: 4 K-80 GPUs on a shared cluster. 
\subsection{Average Runtimes}
\begin{table}[]
\begin{tabular}{ccc}
\textbf{Model} & \textbf{Task}           & \textbf{Time}                                                     \\
\textit{CRQA}  & \textit{Training}       & \textit{\begin{tabular}[c]{@{}c@{}}9.5 hrs\\ /epoch\end{tabular}} \\
\textit{SpNet} & \textit{Training}       & \textit{\begin{tabular}[c]{@{}c@{}}10 hrs/\\ epoch\end{tabular}}  \\
\textit{CRQA}  & \textit{Dev-test}       & \textit{60 hrs}                                                   \\
\textit{SpNet} & \textit{Dev-test}       & \textit{60 hrs}                                                   \\
\textit{CRQA}  & \textit{Dev-test-small} & \multicolumn{1}{l}{5.0 hrs}                                       \\
\textit{SpNet} & \textit{Dev-test-small} & \multicolumn{1}{l}{5.5 hrs}                                       \\
\textit{CRQA}  & \textit{Test}           & \textit{60 hrs}                                                   \\
\textit{SpNet} & \textit{Test}           & \textit{60 hrs}                                                  
\end{tabular}
\end{table}

\begin{table}[H]
\begin{tabular}{cc}
\textbf{Model}                                                         & \textbf{\#param} \\
\textit{CRQA}                                                          & \textit{3M}      \\
\textit{SpNet}                                                         & \textit{3M}      \\
\textit{\begin{tabular}[c]{@{}c@{}}Spatio-Textual\\ CRQA\end{tabular}} & \textit{6.8M}   
\end{tabular}
\end{table}

\begin{table}[H]
\centering
\begin{tabular}{|l|l|}
\hline
\multicolumn{1}{|c|}{\textbf{Model}} & \multicolumn{1}{c|}{\textbf{No. of parameters}} \\ \hline
SpNet w/o DRL & 81.8K \\ \hline
SpNet & 81.8K \\ \hline
BERT SpNet w/o DRL & 109.7M \\ \hline
BERT SpNet & 109.7M \\ \hline
\end{tabular}
\caption{} 
\label{tab:toy-param-table}
\end{table}

\begin{table}[H]
\scriptsize
\centering
\begin{tabular}{|l|l|l|l|l|l|l|}
\hline
\multicolumn{1}{|c|}{\textbf{}} & \multicolumn{2}{c|}{\textbf{Automated evaluation}} & \multicolumn{2}{c|}{\textbf{Human evaluation}} \\ \hline
\multicolumn{1}{|c|}{\textbf{}} & \multicolumn{1}{c|}{\textbf{Location}} & \multicolumn{1}{c|}{\textbf{Non-location}} & \multicolumn{1}{c|}{\textbf{Location}} & \multicolumn{1}{c|}{\textbf{Non-location}} \\ \hline
$\csr$ & 28.00 & 36.00 & 64.00 & 70.00  \\  \hline
\begin{tabular}[c]{@{}c@{}}Spatio-textual\\ CSRQA\end{tabular} 
& 32.00 & 32.00 & 84.00 & 72.00 \\ \hline
\end{tabular}
\caption{} 
\label{tab:error-main-table}
\end{table}

\begin{table*}
\scriptsize
\centering
\begin{tabular}{|l|l|}
\hline
\multicolumn{1}{|c|}{\textbf{Id}} & \multicolumn{1}{c|}{\textbf{Description}} \\ \hline
1 & Do you have any recommendations of \textit{ENTITY} near the \textit{LOCATION}? \\ \hline
2 & Does anyone have ideas on \textit{ENTITY} close to \textit{LOCATION}? Thank you! \\ \hline
3 & Hello! Could anyone please suggest \textit{ENTITY} in the neighborhood of \textit{LOCATION}? \\ \hline
4 & Good Morning! Can someone please propose \textit{ENTITY} not very far from \textit{LOCATION}? \\ \hline
5 & I once lived around \textit{LOCATION}. Does anyone have ideas of \textit{ENTITY} close to the \textit{LOCATION}? Thanks! \\ \hline
6 & Any nice suggestions of \textit{ENTITY} near the \textit{LOCATION}? I will be going to \textit{LOCATION} the next day. \\ \hline
7 & I just came from \textit{LOCATION}. Someone, please recommend \textit{ENTITY} in the neighborhood of \textit{LOCATION}. \\ \hline
8 & Could anyone propose \textit{ENTITY} not far from the \textit{LOCATION}? I need to leave for \textit{LOCATION} urgently. \\ \hline
9 & Any suggestions for \textit{ENTITY} quite far from the \textit{LOCATION}? Thank you very much! \\ \hline
10 & Somebody please suggest \textit{ENTITY} cut off from \textit{LOCATION}. Have a good day! \\ \hline
11 & Does anyone have suggestions for \textit{ENTITY} away from \textit{LOCATION}? Thanks a lot! \\ \hline
12 & Good Afternoon! Any proposals for \textit{ENTITY} not very close to the \textit{LOCATION}? \\ \hline
13 & Hey! I will be staying at \textit{LOCATION}. Please suggest \textit{ENTITY} cut off from \textit{LOCATION}. \\ \hline
14 & Any pleasant ideas of \textit{ENTITY} far off the \textit{LOCATION}? I might then be visiting \textit{LOCATION}. \\ \hline
15 & I came from \textit{LOCATION} this afternoon. Any proposal for \textit{ENTITY} not close to the \textit{LOCATION}? \\ \hline
16 & Does anyone have a suggestion for \textit{ENTITY} distant from \textit{LOCATION}? By the way, I came from \textit{LOCATION} yesterday. \\ \hline
17 & Suggestions for \textit{ENTITY} close to both \textit{LOCATION} and \textit{LOCATION}? \\ \hline
18 & Some good ideas of \textit{ENTITY} between \textit{LOCATION} and \textit{LOCATION}? Thanks much! \\ \hline
19 & Please advise \textit{ENTITY} close to \textit{LOCATION} and not very far off the \textit{LOCATION}. \\ \hline
20 & Any ideas for \textit{ENTITY} near \textit{LOCATION} and also close to \textit{LOCATION} would be welcomed? \\ \hline
21 & We came from \textit{LOCATION} this morning. Suggestions for \textit{ENTITY} close to both \textit{LOCATION} and \textit{LOCATION}? \\ \hline
22 & Any ideas of \textit{ENTITY} between \textit{LOCATION} and \textit{LOCATION}? I would be going to \textit{LOCATION}. Thanks. \\ \hline
23 & We might be staying around \textit{LOCATION}. Please advise \textit{ENTITY} close to \textit{LOCATION} and not far from \textit{LOCATION}. \\ \hline
24 & Could anyone suggest ideas for \textit{ENTITY} close to \textit{LOCATION} and around \textit{LOCATION}? We could be going to \textit{LOCATION} soon. \\ \hline
25 & Suggestions on \textit{ENTITY} far from both \textit{LOCATION} and \textit{LOCATION}? Thank! \\ \hline
26 & Hi! Any idea of \textit{ENTITY} far away from \textit{LOCATION} and \textit{LOCATION}? \\ \hline
27 & Could anyone please propose \textit{ENTITY} not close to \textit{LOCATION} and also far from \textit{LOCATION}? \\ \hline
28 & Does anyone have any suggestions for \textit{ENTITY} far from \textit{LOCATION} and not around \textit{LOCATION}? \\ \hline
29 & We will be staying near the \textit{LOCATION}. Suggestions for \textit{ENTITY} far from both \textit{LOCATION} and \textit{LOCATION} will be welcomed. \\ \hline
30 & Any idea of \textit{ENTITY} far away from \textit{LOCATION} and \textit{LOCATION}? I would then be visiting \textit{LOCATION}. \\ \hline
31 & Hi, I will be staying near the \textit{LOCATION}. Could anyone propose \textit{ENTITY} not very close to \textit{LOCATION} and far from \textit{LOCATION}? \\ \hline
32 & Does anyone have suggestions for \textit{ENTITY} far from \textit{LOCATION} and also far from \textit{LOCATION}? I will then be visiting \textit{LOCATION} too. \\ \hline
33 & Any good ideas of \textit{ENTITY} far from \textit{LOCATION} but close to \textit{LOCATION} would be appreciated? Best Regards. \\ \hline
34 & Anyone having ideas of \textit{ENTITY} close to \textit{LOCATION} but far from \textit{LOCATION}? \\ \hline
35 & Someone please advise \textit{ENTITY} far from \textit{LOCATION} but not very far from \textit{LOCATION}. \\ \hline
36 & Suggest \textit{ENTITY} close to \textit{LOCATION} but not in the neighborhood of \textit{LOCATION}. Thank you so much! \\ \hline
37 & Does anyone have good ideas of \textit{ENTITY} far from \textit{LOCATION} but near \textit{LOCATION}? Regards. \\ \hline
38 & Please suggest ideas of \textit{ENTITY} in the neighborhood of \textit{LOCATION} but far from \textit{LOCATION}. \\ \hline
39 & Could anyone advise \textit{ENTITY} far from \textit{LOCATION} but not too far from \textit{LOCATION}? \\ \hline
40 & Any nice ideas of \textit{ENTITY} close to \textit{LOCATION} but not in the neighborhood of \textit{LOCATION}. Thanks! \\ \hline
41 & Tomorrow, I would be coming to stay at \textit{LOCATION}. Anyone having ideas of \textit{ENTITY} close to \textit{LOCATION} but far from \textit{LOCATION}? \\ \hline
42 & Please propose \textit{ENTITY} far from \textit{LOCATION} but not far from \textit{LOCATION}. I will then be exploring \textit{LOCATION}. \\ \hline
43 & I came from \textit{LOCATION} this evening. Any nice ideas for \textit{ENTITY} far from \textit{LOCATION} but close to \textit{LOCATION} would be appreciated?  \\ \hline
44 & Suggest \textit{ENTITY} close to \textit{LOCATION} but not near \textit{LOCATION}. Tomorrow, I will be leaving for \textit{LOCATION}. \\ \hline
45 & Yesterday, I came to stay at \textit{LOCATION}. Any ideas of \textit{ENTITY} close to \textit{LOCATION} but far from \textit{LOCATION}? \\ \hline
46 & Suggestions of \textit{ENTITY} far from \textit{LOCATION} but not very far from \textit{LOCATION}. I will then be moving to \textit{LOCATION}. \\ \hline
47 & I came from \textit{LOCATION} today. Any good ideas for \textit{ENTITY} far from \textit{LOCATION} but near to \textit{LOCATION} would be welcomed?  \\ \hline
48 & Advise \textit{ENTITY} close to \textit{LOCATION} but not close to \textit{LOCATION}. I might be leaving for \textit{LOCATION} soon. \\ \hline
\end{tabular}
\caption{} 
\label{tab:toy-param-table}
\end{table*}
